# Supplementary material for: DevFormer: A Symmetric Transformer for Context-Aware Device Placement
Source: arXiv:2205.13225 source file (2023-06-07)
Supplement: Supplementary file 1 [file appendix_D.tex]

\section{Details of Neural Architecture Design}
\label{append: neural_architecture}

Our neural architecture has the AM \citep{kool_attention} with context modification. The AM is a transformer\citep{transformer}-based encoder-decoder model designed to solve combinatorial optimization problems. We used conventional notations from transformer \citep{transformer} and AM \citep{kool_attention}, including multi-head attention (MHA), feed forward (FF), query, key and value ($Q,K,V$). Because their terminologies are well organized, we tried to keep every notation as possible. In this paper, we focused on presenting the main differences between AM and our architecture. See \citet{kool_attention} for detailed mechanism of AM.

\subsection{Change of Notations.} 
\label{append: notation}
There are small revisions we made from \citet{kool_attention}. In AM, TSP nodes are presented as $\boldsymbol{x}_i$, $i\in \{1,...,N\}$, where $N$ refers to the number of TSP nodes. This paper uses $I_{probe}$ for the node of the probing port, $I_{keepout}$ for nodes of the keep-out regions and $I_{allowed}$ for nodes of the decap-allowed ports. 

\citet{kool_attention} denotes action as $\boldsymbol{\pi}$ (for representing permutation action), but we denoted action as $\boldsymbol{a}$. 

In, \citet{kool_attention}, the notation, $\boldsymbol{h}^{(N)}$, refers to $N$ times MHA in encoder; we denoted this notation as $\boldsymbol{h}$ just for readability.

There are two additional notations: $\boldsymbol{c}_{probe}$ is the probing context embedding from the probing port context network (PCN in section \hyperlink{subsection.3.2}{3.2}) and $\boldsymbol{c}_{a_{t-1}}$ is the recurrent context embedding from the recurrent context network (RCN in section \hyperlink{subsection.3.2}{3.2}) for $step=t$.

\begin{figure}[h]
\centerline{\includegraphics[width=1\textwidth]{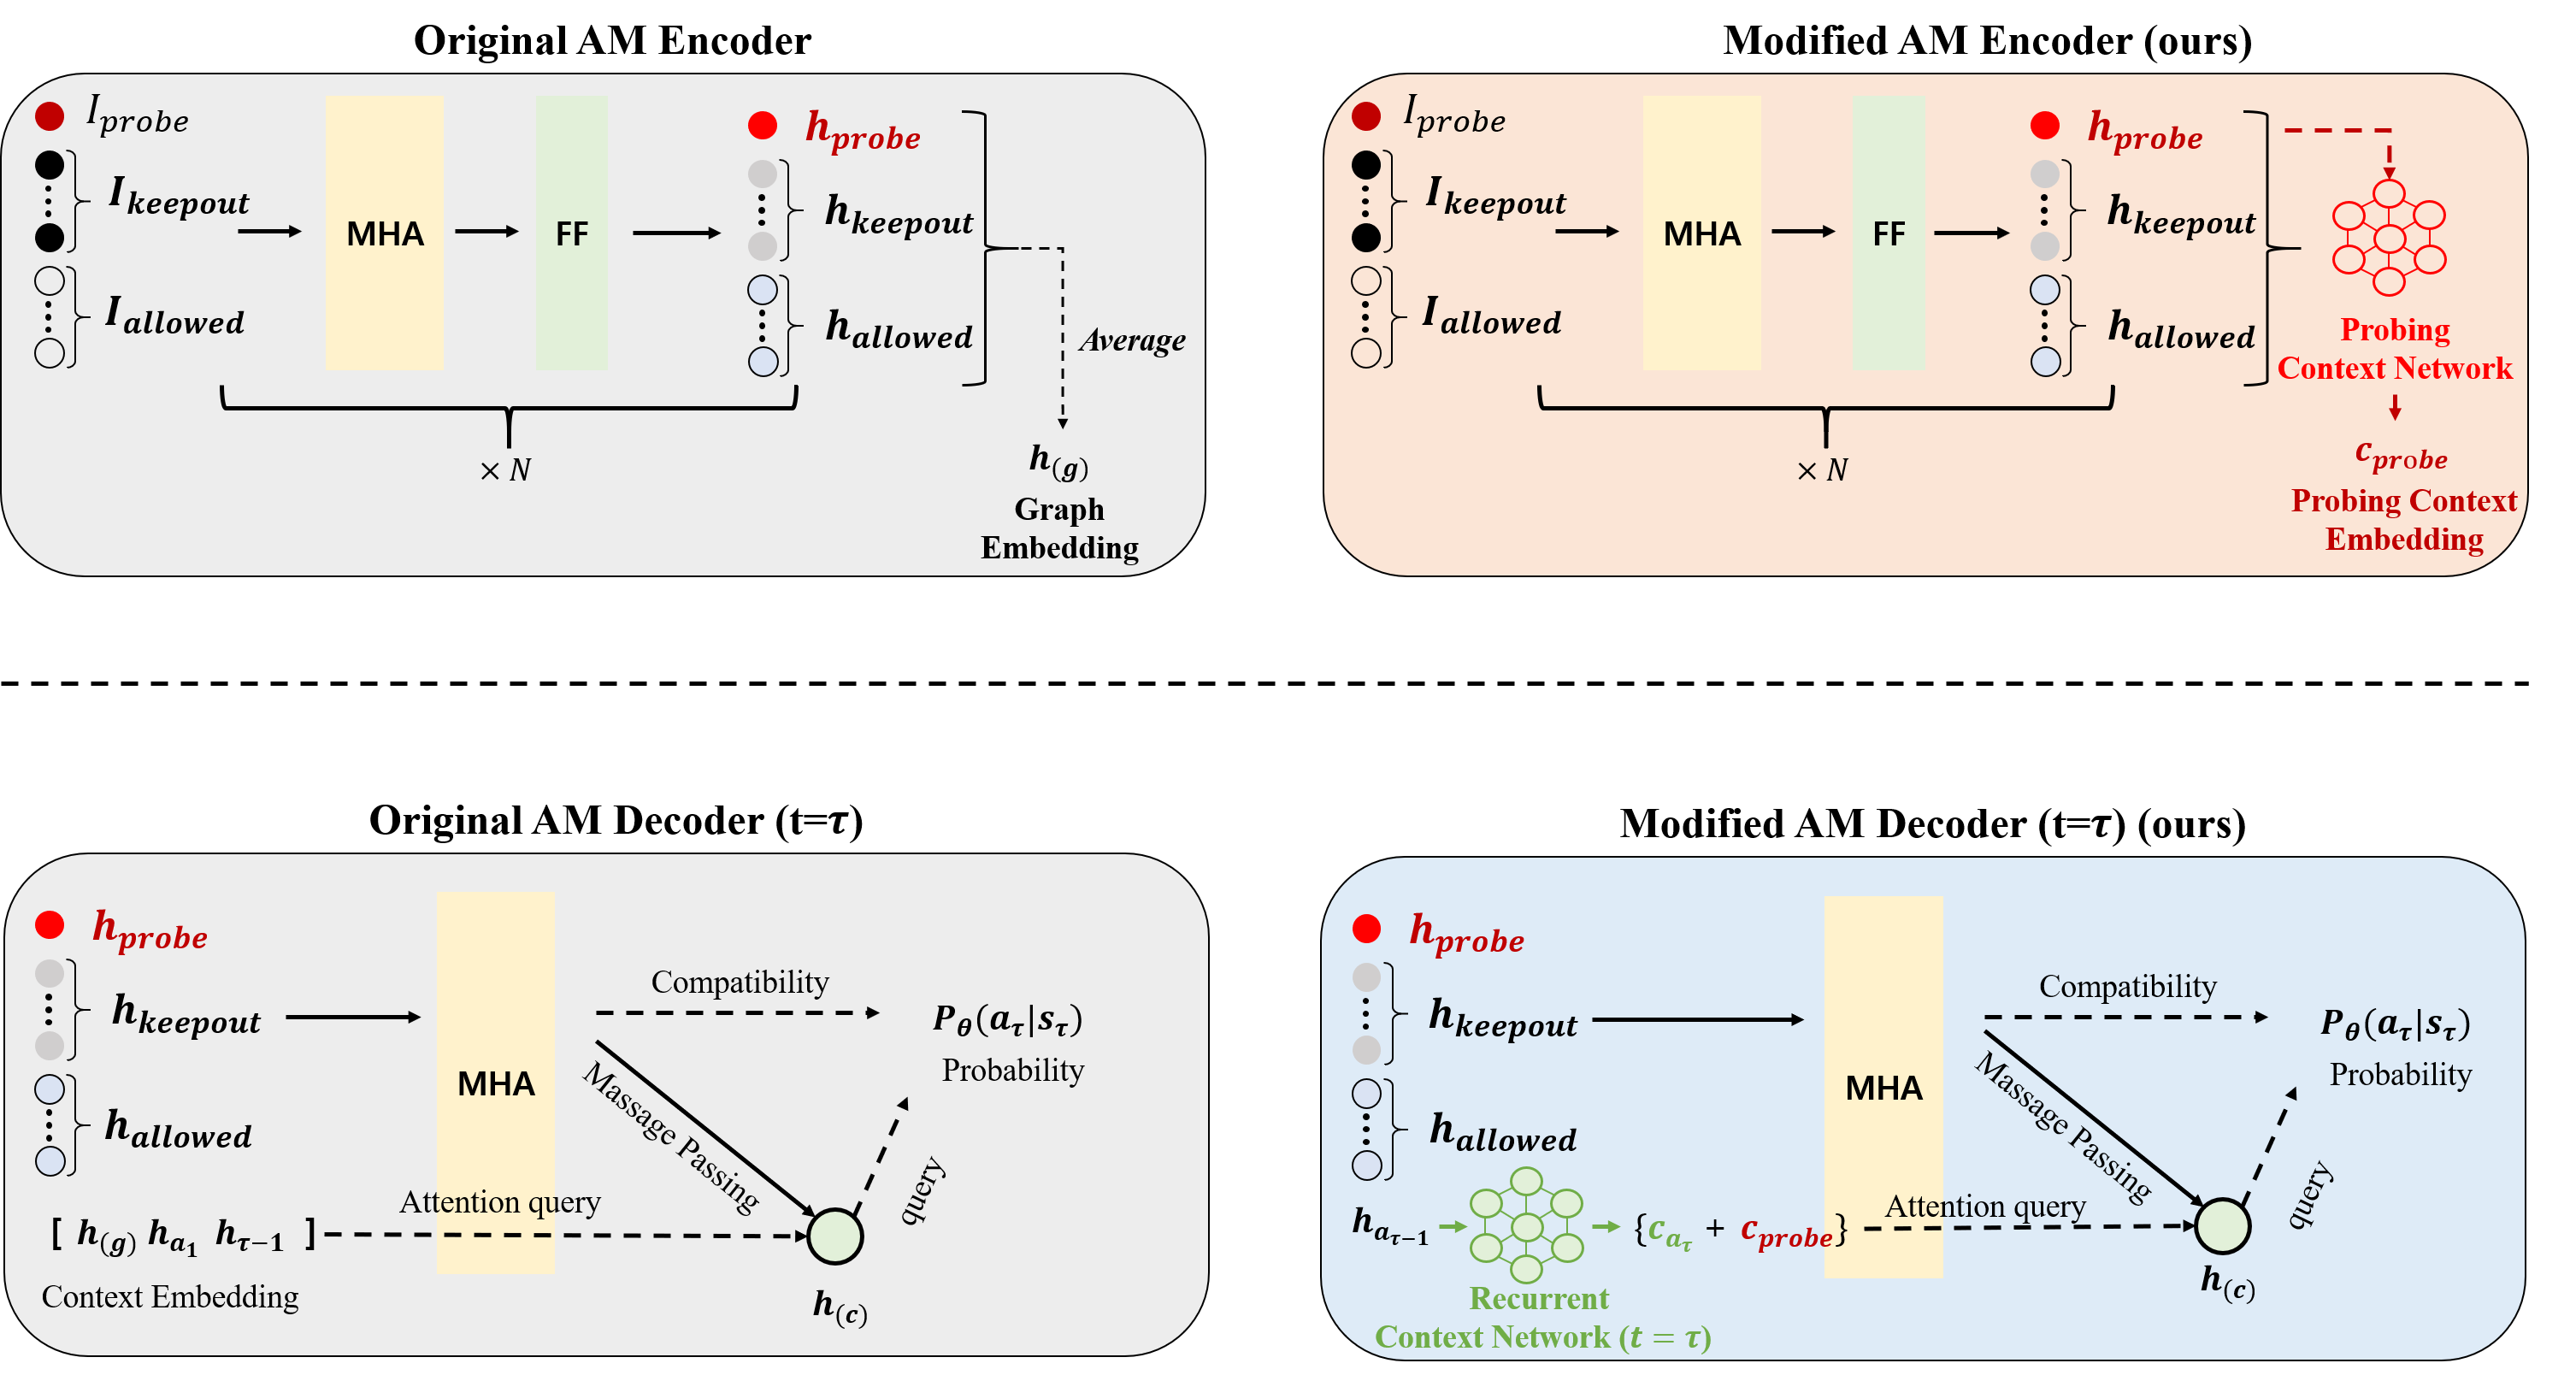}}
\caption{Overview of main difference between AM and modified version of AM.}
\label{neural_architecture}
\end{figure}

\subsection{Highlight of modifications: Context Embedding.}
\label{append: context-modification}
The main difference between the AM and ours is the context embedding and is illustrated in \cref{neural_architecture}. 

AM's \citep{kool_attention} context embedding is presented as follows: 
\begin{equation}
    \boldsymbol{{h}_{(c)}} = {MHA}([\boldsymbol{{h}_{(g)}}, \boldsybol{{h}_{a_{\tau-1}}},\boldsymbol{{h}_{a_1}}],\boldsymbol{h})
\end{equation}

\textbf{Context embedding of AM.} Since the AM was originally designed for TSP and its invariant problems, AM's context embedding is implemented for capturing the entire graph by taking the average of all node embedding, $\boldsymbol{{h}_{(g)}}$, state-transition with $\boldsymbol{{h}_{a_{\tau-1}}}$ and final destination with $\boldsymbol{{h}_{a_1}}$. Note that TSP is a routing problem, where it must return to the first node (i.e, destination node is first visited node).

\textbf{Context embedding of AM for DPP (AM-CRL \citep{hyunwook_decap}).} \citet{hyunwook_decap} also used the AM for decap placement with modification of context embedding. \citet{hyunwook_decap} tried to add $\boldsymbol{{h}_{probe}}$ to capture the location of probing port as follows:

\begin{equation}
    \boldsymbol{{h}_{(c)}} = {MHA}([\boldsymbol{{h}_{(g)}}, \boldsymbol{{h}_{a_{t-1}}},\boldsymbol{{h}_{p}}], \boldsymbol{h})
\end{equation}

\textbf{Context embedding of Ours.} We observed that $\boldsymbol{{h}_{(g)}}$ degrades the performance of the model for DPP. DPP is different from TSP; we need a new DPP-specific context embedding strategy. Therefore, we tried to focus on the probing port more than others by proposing the PCN. We removed $\boldsymbol{{h}_{(g)}}$ and $\boldsymbol{{h}_{a_1}}$ from the context embedding and replaced them with our newly designed context embedding. Our context embedding is described as follows:

\begin{equation}
    \boldsymbol{{h}_{(c)}} = {MHA}(\boldsymbol{c_{probe}} + \boldsymbol{{c}_{a_{t-1}}},\boldsymbol{h})
\end{equation}
\begin{equation}
    \boldsymbol{{c}_{probe}} = \textbf{MLP}_{PCN} (\boldsymbol{{h}_{probe}}) 
\end{equation}
\begin{equation}
    \boldsymbol{{c}_{a_{t-1}}}  = \textbf{MLP}_{RCN} (\boldsymbol{{h}_{a_{t-1}}} ) 
\end{equation}

Note that both $\textbf{MLP}_{PCN}$ and $\textbf{MLP}_{RCN}$ are two-layer perceptron models with ReLU activation, where input and output dimensions are identical ($d = 128$ in all experiments).

\subsection{Calculation of Probability.}
\label{append: prob}

Probability calculations using context hidden embedding $\boldsymbol{h}_{(c)}$, and PDN hidden embedding $\boldsymbol{h}_i$, $i\in \{1,...,N_{row} \times N_{col} \}$ in (11-14) are exactly identical to (5-8) in \citet{kool_attention} except the masking mechanism in \eqref{mask1} and \eqref{mask2}. Because \citet{kool_attention} solves TSP, so they mask the previously selected actions by forcing $-\infty$ as compatibility $u_{(c)j}$. For DPP, we mask not only the previously selected actions $\boldsymbol{a}_{1:t-1}$ but also the probing port index $I_{probe}$ and the keep-out region indices $I_{keepout}$; it is forbidden to choose the $I_{probe}$, $I_{keepout}$ and previously selected actions $a_{1:t-1}$

Query, key and value are computed by:

\begin{equation}
    \boldsymbol{q}_{c} = W^{Q}\boldsymbol{h}_{(c)},\boldsymbol{k}_{i} = W^{K}\boldsymbol{h}_{i},\boldsymbol{v}_{i} = W^{V}\boldsymbol{h}_{i}
\end{equation}

Note that $W^{Q}$, $W^{K}$ and $W^{V}$ are 128-to-128 linear projections.

After that, compatibility $u_{(c) j}$ is computed by the dot product of query and key, with masking mechanism (setting $-\infty$ not to select actions in $\boldsymbol{s}_{t-1}$).

\begin{equation}
u_{(c) j}= \begin{cases}\frac{\mathbf{q}_{(c)}^{T} \mathbf{k}_{j}}{\sqrt{128}} & \text { if } j \notin I_{probe}, I_{keepout}, a_{1:t-1} \\ -\infty & \text { otherwise }\end{cases}
\label{mask1}
\end{equation}

The $tanh$ clipping is done following \citet{bello_pointer} and \citet{kool_attention}. 

\begin{equation}
    u_{(c) j}= \begin{cases}10 \cdot \tanh \left(\frac{\mathbf{q}_{(c)}^{T} \mathbf{k}_{j}}{\sqrt{128}}\right) & \text { if } j \notin I_{probe}, I_{keepout}, a_{1:t-1} \\ -\infty & \text { otherwise. }\end{cases}
\label{mask2}
\end{equation}

Finally, probability can be computed using softmax function as follows:

\begin{equation}
    p_{\boldsymbol{\theta}}\left(a_{t}=i \mid \boldsymbol{s}_{t} \right)=\frac{e^{u_{(c) i}}}{\sum_{j} e^{u_{(c) j}}}
\end{equation}
