# Supplementary material for: DevFormer: A Symmetric Transformer for Context-Aware Device Placement
Source: arXiv:2205.13225 source file (2023-06-07)
Supplement: Supplementary file 2 [file GA_additional.tex]

\begin{table}[h!]
\fontsize{9}{9}\selectfont
\begin{center}
\caption{{Ablation study on genetic algorithm with different operator values.}}
\label{Table01}
\begin{tabular}{cccc}
\specialrule{1.0pt}{0pt}{4pt}
PI Simulation ($M$) & Population Size ($P$) & Generations ($G$) & Avg. Score\\
\specialrule{1.0pt}{0pt}{4pt}
\begin{tabular}{c}
\multirow{3}{*}{1000}
\end{tabular}
& 50 & 20 & 12.61\\
& 100 & 10 & 12.82\\
& 200 & 5 & 12.79\\

\specialrule{0.5pt}{0pt}{4pt}
\begin{tabular}{c}
\multirow{4}{*}{2000}
\end{tabular}

& 50 & 40 & 12.37\\
& 100 & 20 & 12.84\\
& 200 & 10 & 12.83\\
& 400 & 5 & 12.80\\

\specialrule{1.0pt}{0pt}{4pt}
\end{tabular}
\end{center}
\vspace{-2mm}
\end{table}
