# Supplementary material for: DevFormer: A Symmetric Transformer for Context-Aware Device Placement
Source: arXiv:2205.13225 source file (2023-06-07)
Supplement: Supplementary file 5 [file C_PI.tex]

The objective of DPP is to suppress impedance of the probing port as much as possible and is measured by the performance metric, \eqref{reward} in chapter 4.1. \textit{CDML} was evaluated in comparison to GA $\{M=100\}$ (\textit{expert policy}), GA $\{M=500\}$, RS $\{M=10,000\}$, AM-RL and AM-IL on 100 test data. Each method was asked to place 20 decaps ($K=20$) on each test.

\subsection{Impedance Suppression over a given Frequency range}
\vspace{-1mm}

\begin{figure}[h!]
\vspace{-2mm}
\centering  
\subfigure[Test Case 1]{\includegraphics[width=0.47\linewidth]{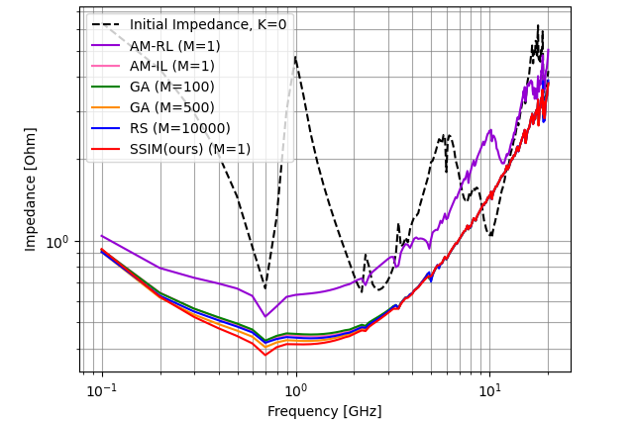}}
\subfigure[Test Case 2]{\includegraphics[width=0.47\linewidth]{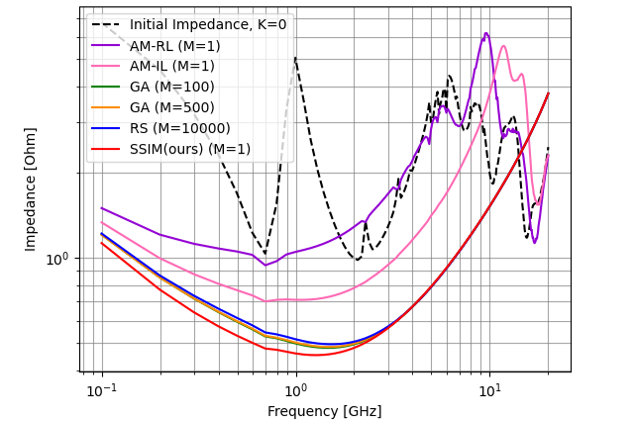}}
\subfigure[Test Case 3]{\includegraphics[width=0.47\linewidth]{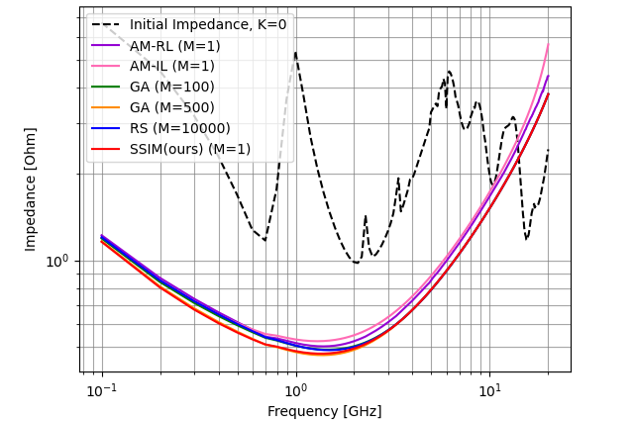}}
\subfigure[Test Case 4]{\includegraphics[width=0.47\linewidth]{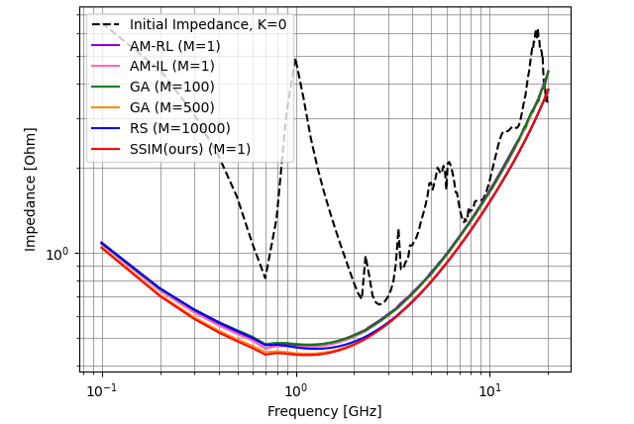}}
\subfigure[Test Case 5]{\includegraphics[width=0.47\linewidth]{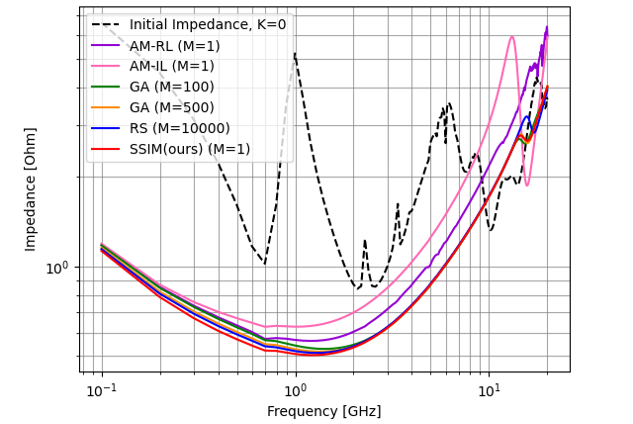}}
\subfigure[Test Case 6]{\includegraphics[width=0.47\linewidth]{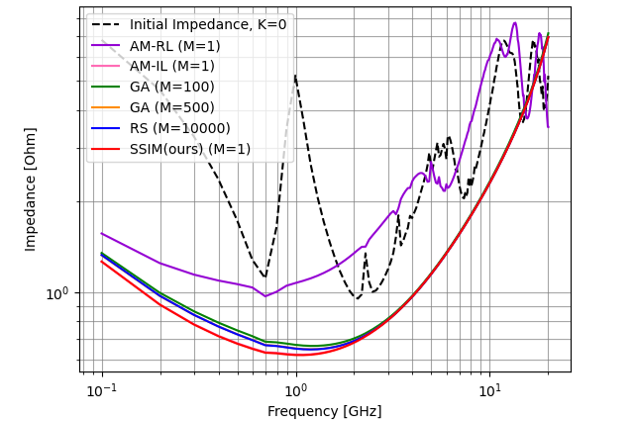}}
\vspace{-2mm}
\caption{Impedance suppressed by each method, GA $\{M=100\}$ (\textit{expert policy}), GA $\{M=500\}$, RS $\{M=10,000\}$, AM-RL , AM-IL and \textit{CDML} (Ours) for 6 example test cases out of 100 test dataset.}
\label{test_cases}
\end{figure}

\clearpage

\subsection{Decap Placement Tendency Illustrations}
\vspace{-2mm}
\begin{figure}[h!]
\centering  
\subfigure[GA $\{M=100\}$ (\textit{expert policy})]{\includegraphics[width=0.85\linewidth]{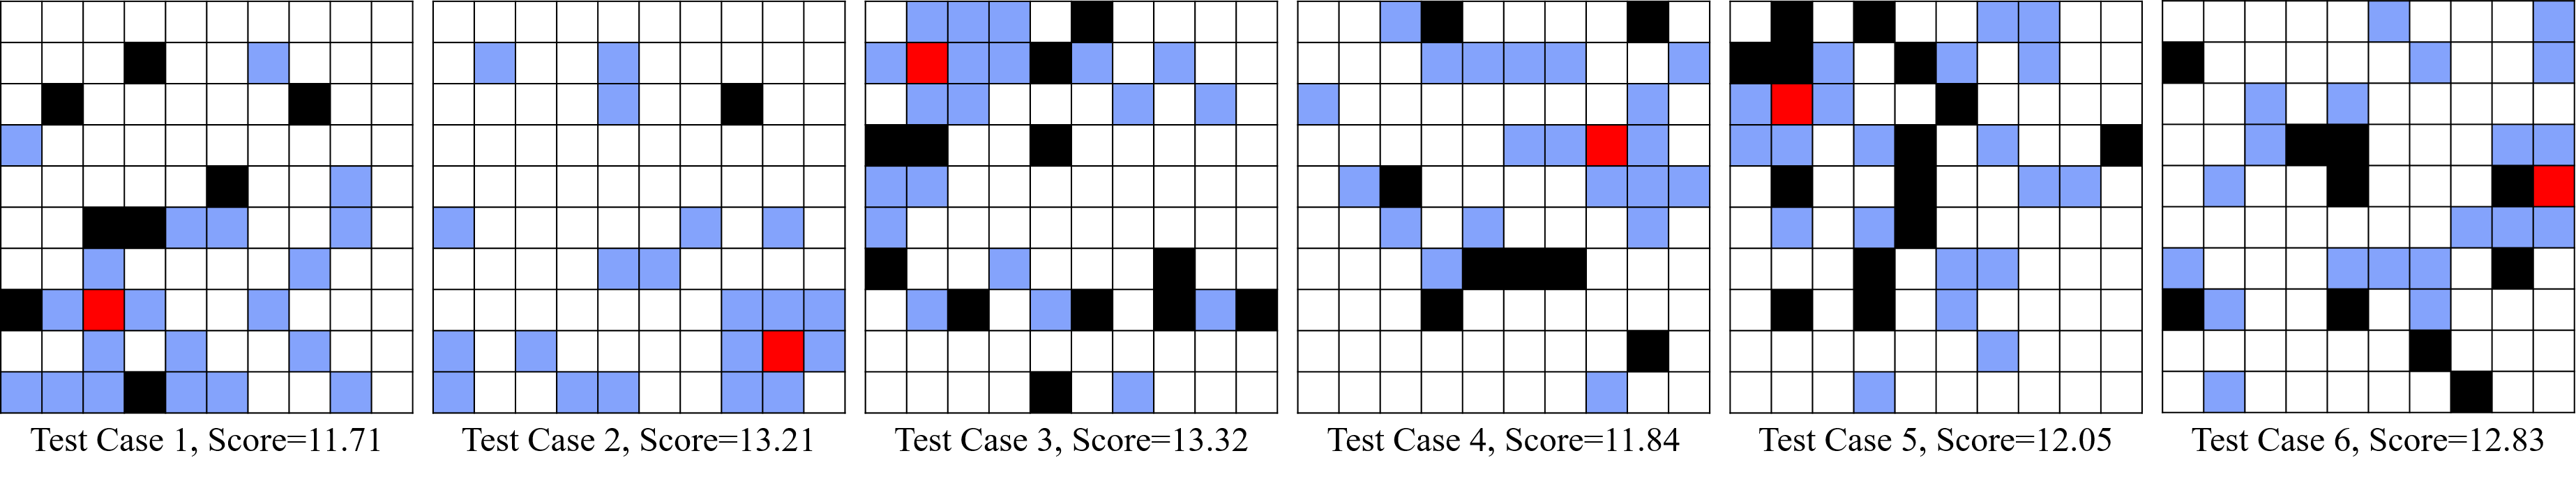}}
\subfigure[GA $\{M=500\}$]{\includegraphics[width=0.85\linewidth]{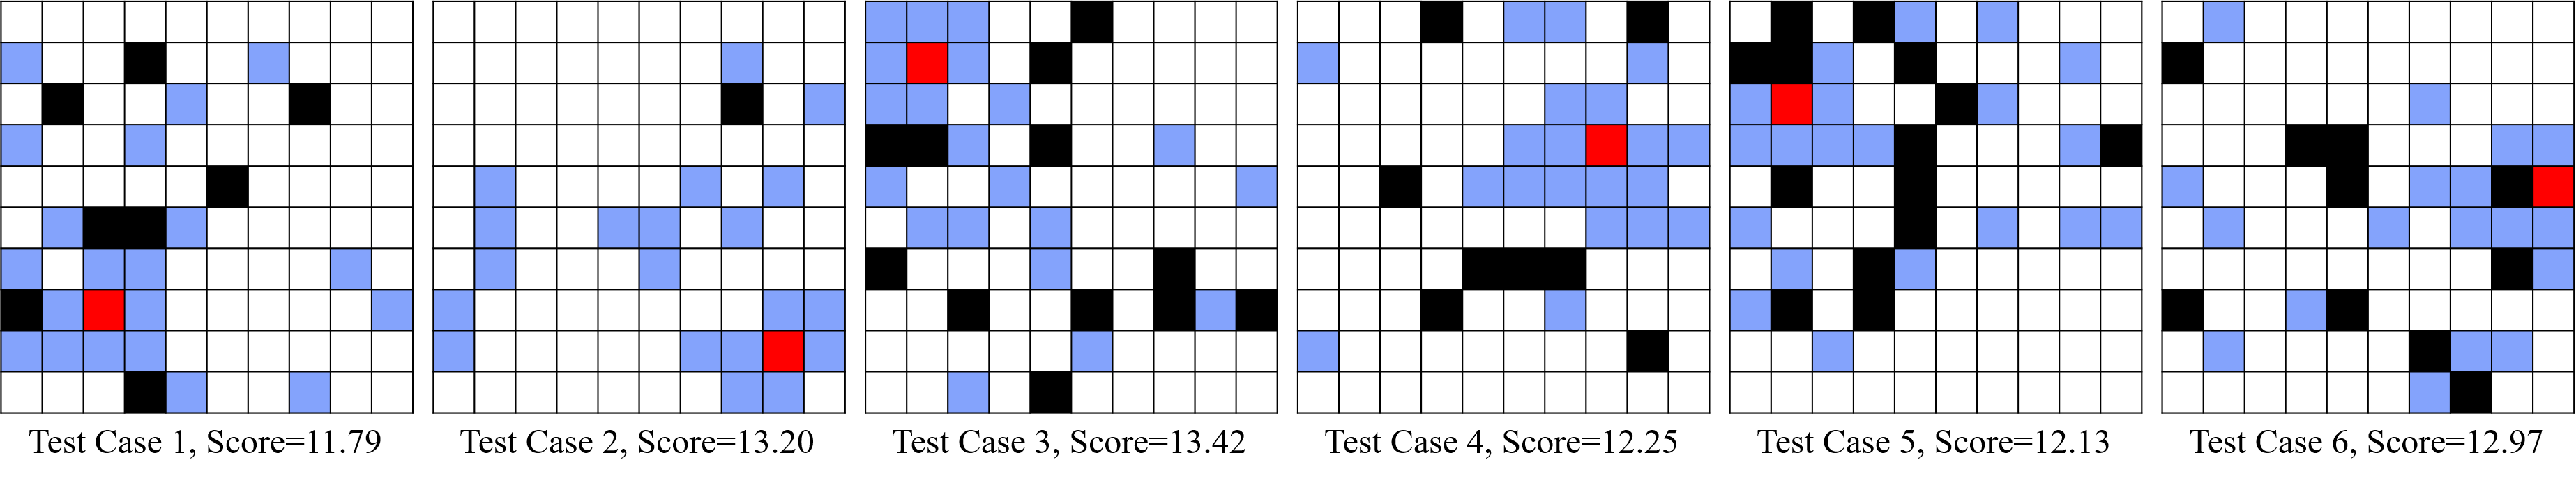}}
\subfigure[RS $\{M=10,000\}$]{\includegraphics[width=0.85\linewidth]{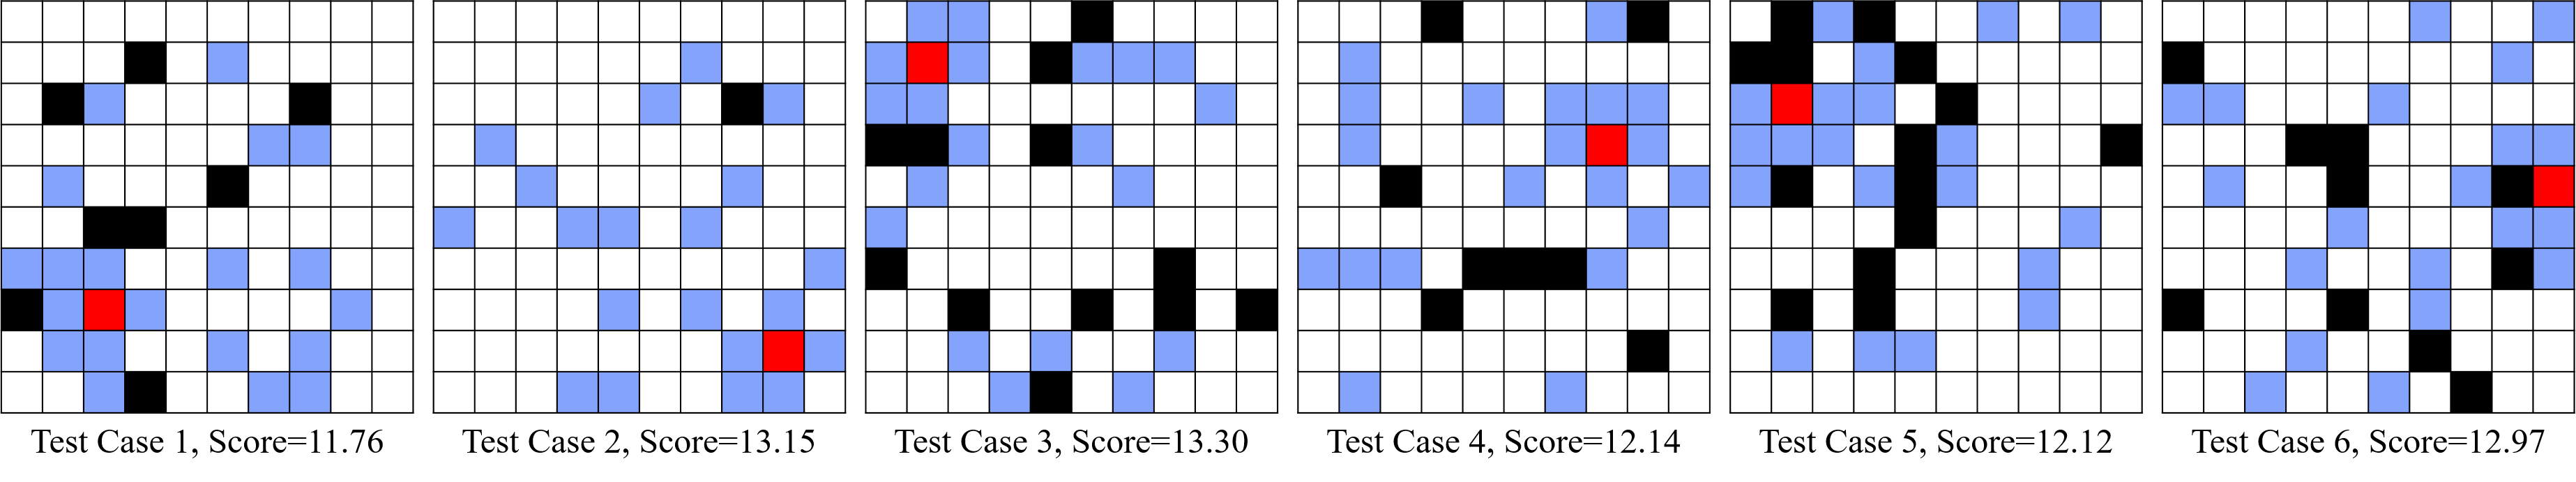}}
\subfigure[AM-RL $\{M=1\}$]{\includegraphics[width=0.85\linewidth]{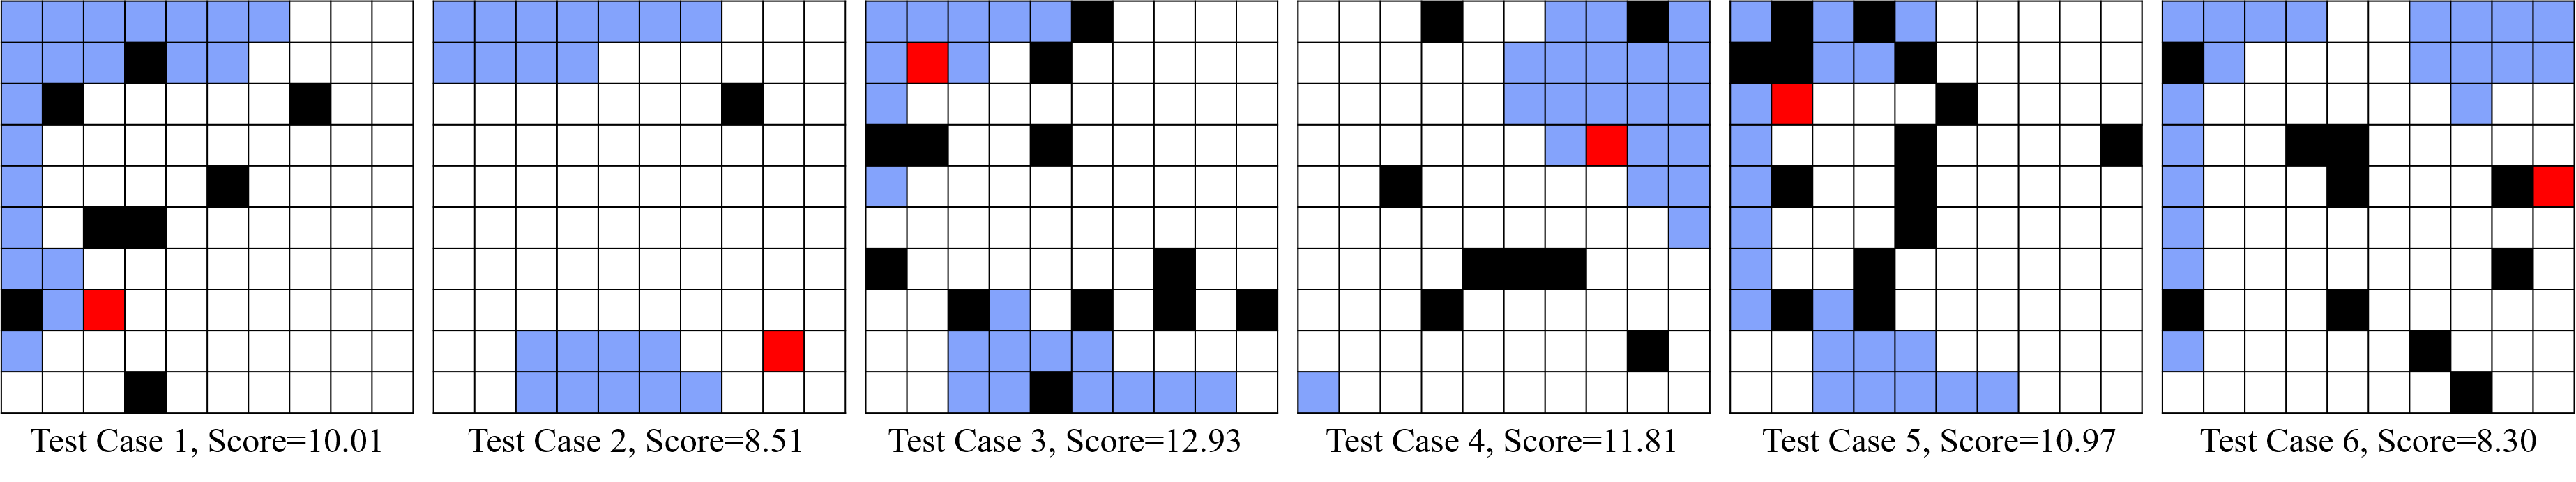}}
\subfigure[AM-IL $\{M=1\}$]{\includegraphics[width=0.85\linewidth]{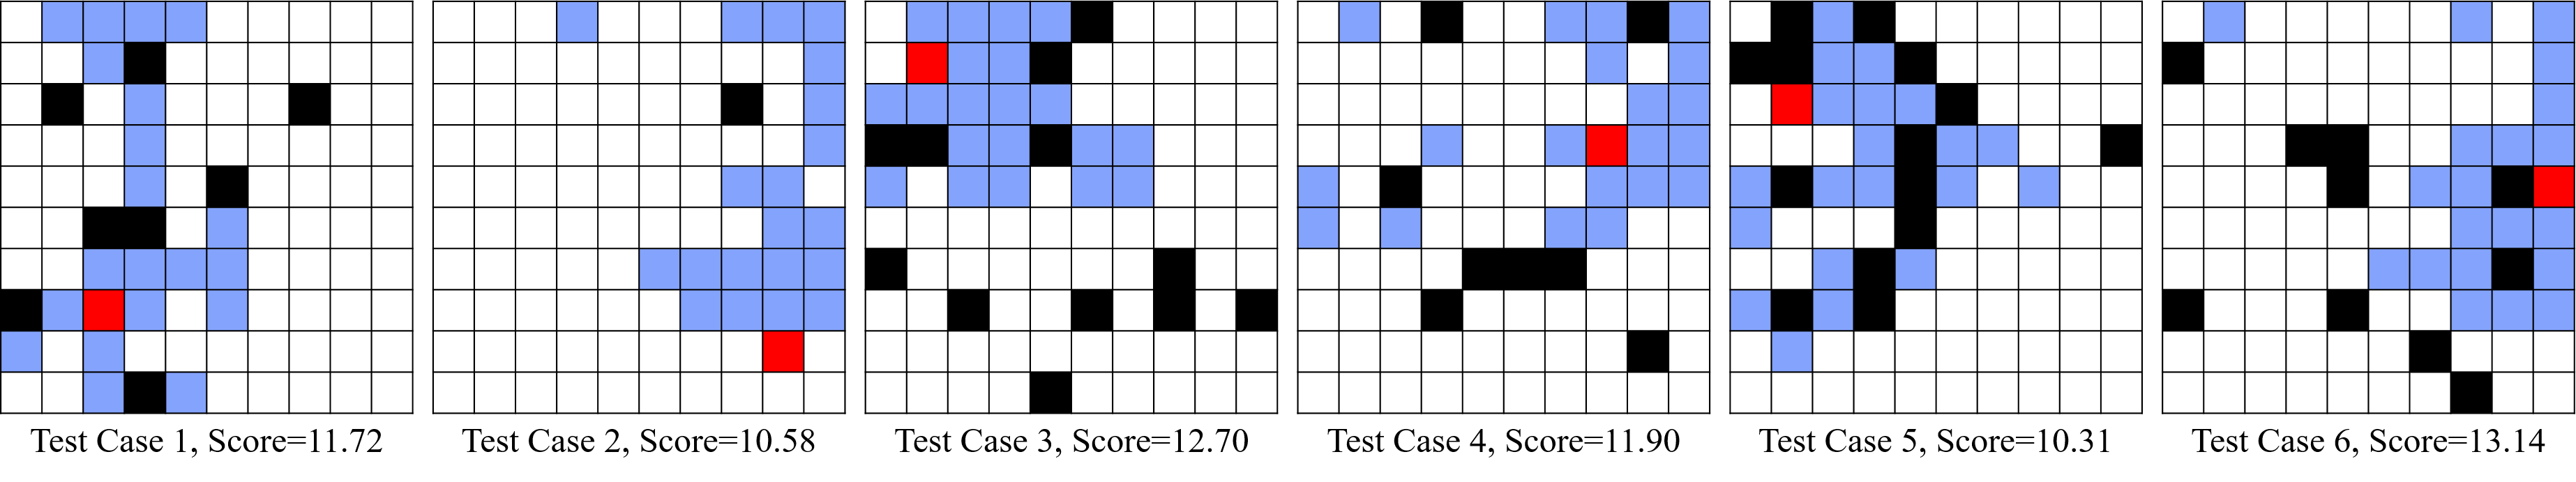}}
\subfigure[\textbf{\textit{CDML (ours)}$\{M=1\}$}]{\includegraphics[width=0.85\linewidth]{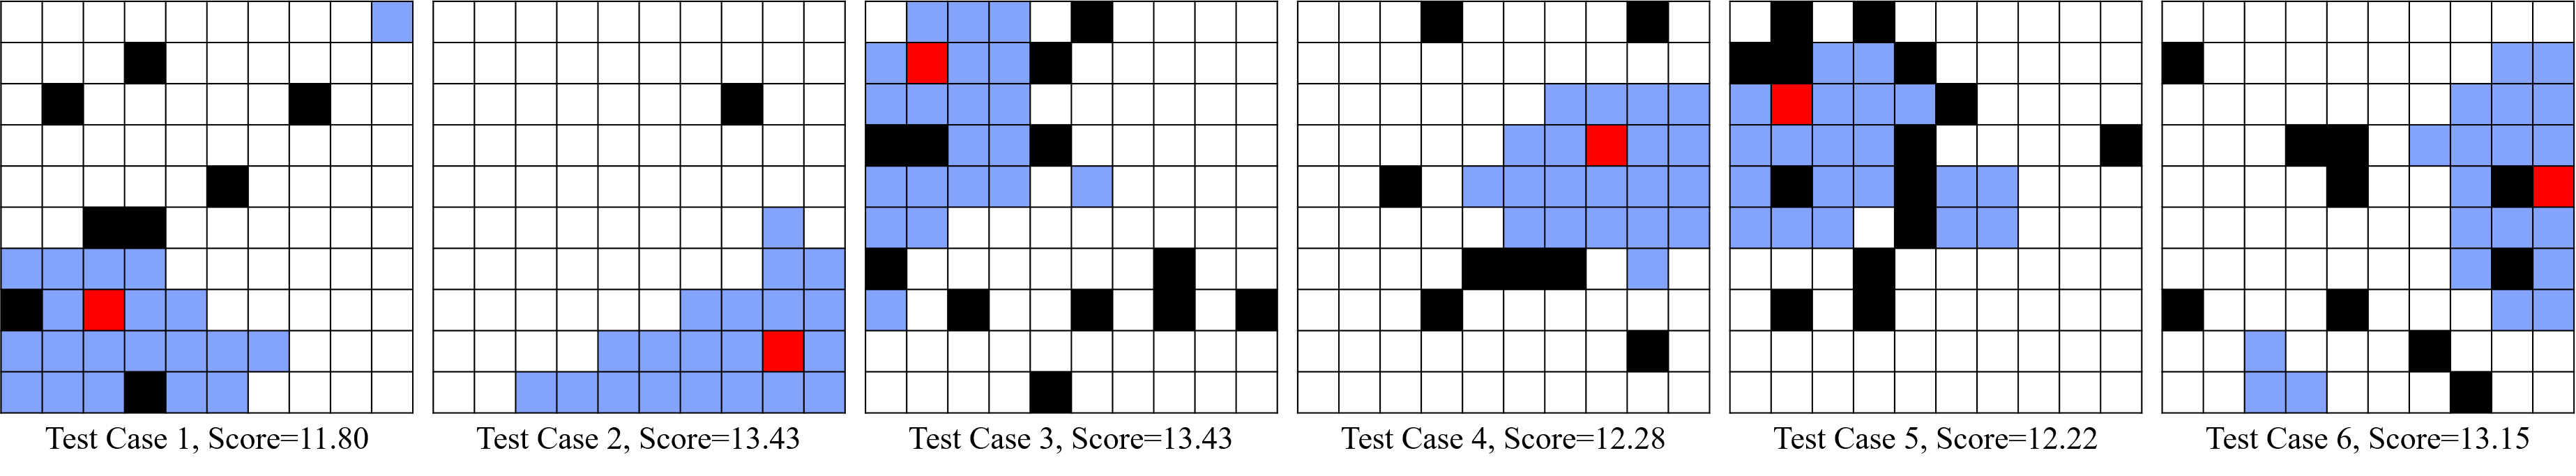}}
\vspace{-3mm}
\caption{Corresponding decap placement solutions to \cref{test_cases} by each method.Red represents probing port, black represents keep-out ports and blue represents decap locations.}
\label{solution}
\vspace{-5mm}
\end{figure}
