# Supplementary material for: DevFormer: A Symmetric Transformer for Context-Aware Device Placement
Source: arXiv:2205.13225 source file (2023-06-07)
Supplement: Supplementary file 6 [file D_Neural.tex]

Our neural architecture has the AM \cite{kool_attention} with context modification. The AM is a transformer\cite{transformer}-based encoder-decoder model designed to solve combinatorial optimization problems. We used conventional notations from transformer \cite{transformer} and AM \cite{kool_attention}, including multi-head attention (MHA), feed forward (FF), query, key and value ($Q,K,V$). Because their terminologies are well organized, we tried to keep every notation as possible. In this paper, we focused on presenting the main differences between AM and our architecture. See \cite{kool_attention} for detailed mechanism of AM.

\subsection{Change of Notations.} There are small revisions we made of \cite{kool_attention}. In AM, TSP nodes are presented as $\boldsymbol{x}_i$, $i\in \{1,...,N\}$, where $N$ refers to the number of TSP nodes. This paper uses $\boldsymbol{x}_p$ for node of the probing port, $\boldsymbol{x}_{1:|\boldsymbol{ko}|}$ for nodes of the keep-out regions and $\boldsymbol{x}_{1:\boldsymbol{d}}$ for nodes of the decap available place. 

\citet{kool_attention} denotes action as $\boldsymbol{\pi}$ (for representing permutation action), but we denoted action as $\boldsymbol{a}$. 

In, \citet{kool_attention}, the notation, $\boldsymbol{h}^{(N)}$, refers to $N$ times MHA in encoder; we denoted this notation as $\boldsymbol{h}$ just for readability.

There are two additional notations: $\boldsymbol{c}_{(p)}$ is the probing context embedding from the probing port context network (PCN in section \hyperlink{subsection.3.2}{3.2}) and $\boldsymbol{c}_{a_{t-1}}$ is the recurrent context embedding from the recurrent context network (RCN in section \hyperlink{subsection.3.2}{3.2}) for $step=t$.


\begin{figure}[h]
\centerline{\includegraphics[width=1\textwidth]{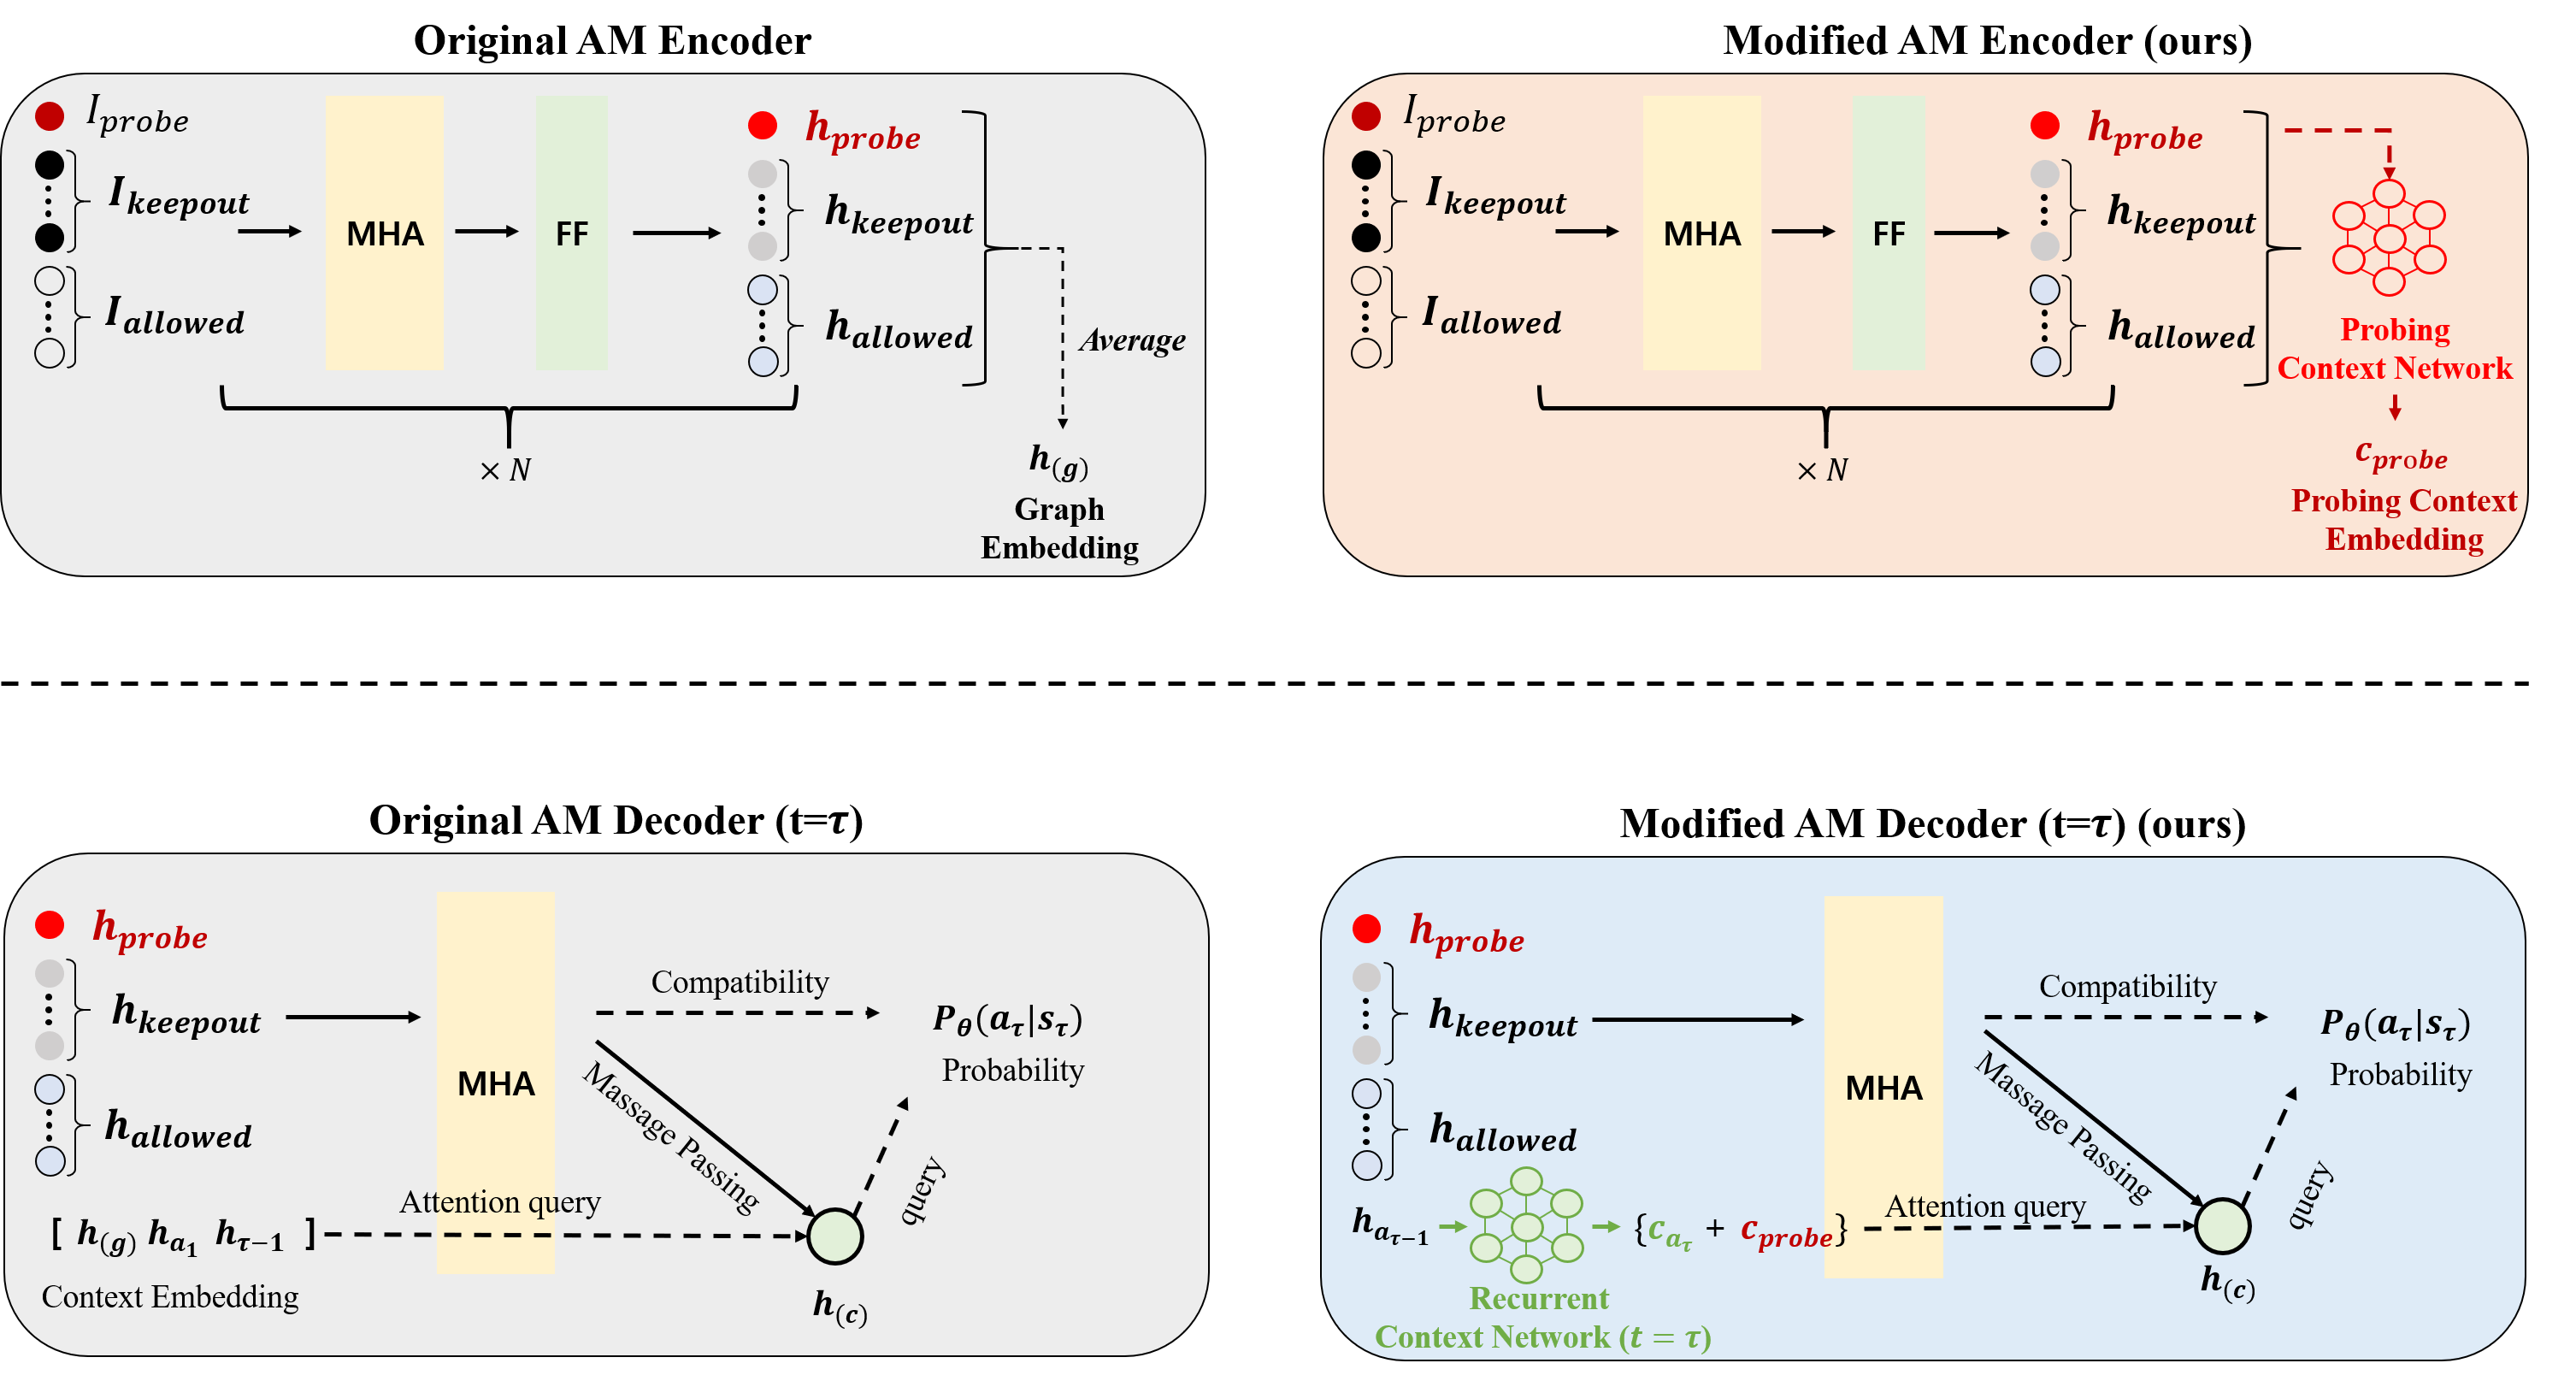}}
\caption{Overview of main difference between AM and modified version of AM.}
\label{neural_architecture}
\end{figure}

\subsection{Highlight of differences: Context Embedding.}

The main highlight of the differences between the AM and ours is context embedding and is presented in \cref{neural_architecture}. 

AM's \cite{kool_attention} context embedding for is presented as follows: 
\begin{equation}
    \textbf{h}_{(c)} = {MHA}([\textbf{h}_{(g)}, \textbf{h}_{a_{\tau-1}},\textbf{h}_{a_1}])
\end{equation}

\textbf{Context embedding of AM.} AM's context embedding is implemented for capturing the entire graph by taking the average of all node embedding, $\textbf{h}_{(g)}$, state-transition with $\textbf{h}_{a_{t-1}}$ and final destination with $\textbf{h}_{a_1}$. Note that TSP is a routing problem, where it must return to the first node (i.e, destination node is first visited node). 



\textbf{Context embedding of AM for DPP (AM-RL \cite{hyunwook_decap}).} \citet{hyunwook_decap} also used AM for decap placement with modification of context embedding. \citet{hyunwook_decap} tried to add $\textbf{h}^p$ to capture the location of probing port as follows:

\begin{equation}
    \textbf{h}_{(c)} = {MHA}([\textbf{h}_{(g)}, \textbf{h}_{a_{t-1}},\textbf{h}_{p}])
\end{equation}



\textbf{Context embedding of Ours.} We observed that $\textbf{h}_{(g)}$ degrades the performance of the model in DPP. DPP is different from TSP; we need a new DPP-specific context embedding strategy. Therefore, we tried to focus on the probing port more than others by proposing PCN. We excluded $\textbf{h}_{(g)}$ and $\textbf{h}_{a_1}$ from the context embedding and replaced them with our newly designed context embedding. Our context embedding is  described as follows:

\begin{equation}
    \textbf{h}_{(c)} = {MHA}(\boldsymbol{c_{(p)}} + \textbf{c}_{a_t}) 
\end{equation}
\begin{equation}
    \textbf{c}_{(p)} = \textbf{MLP}_{PCN} (\textbf{h}_p) 
\end{equation}
\begin{equation}
    \textbf{c}_{a_t}  = \textbf{MLP}_{RCN} (\textbf{h}_{a_t} ) 
\end{equation}

Note that $\textbf{MLP}_{PCN}$ and $\textbf{MLP}_{RCN}$ is a two-layer perceptron with ReLU activation, where input and output dimensions are identical ($d = 128$ in all experiments). 

\subsection{Calculation of Probability.}

Probability calculations using $\boldsymbol{h}_{(c)}$, and $\boldsymbol{h}_i$, $i\in \{1,...,N \times M \}$ in (11-14) are exactly identical to (5-8) in \citet{kool_attention} except the masking mechanism in \eqref{mask1} and \eqref{mask2}. Because \citet{kool_attention} solve TSP, they mask previously selected actions by forcing $-\infty$ as compatibility $u_{(c)j}$. For DPP, we mask not only the previously selected actions $\boldsymbol{a}_{1:t-1}$, but also probing index $p$ and keep-out region indices $\boldsymbol{ko}$; it is forbidden to choose the indices in current state $\boldsymbol{s_{t-1}} = \{ p,\boldsymbol{ko},\boldsymbol{a}_{1:t-1} \} $. 

Query, key and value are computed by:

\begin{equation}
    \boldsymbol{q}_{c} = W^{Q}\boldsymbol{h}_{(c)},\boldsymbol{k}_{i} = W^{K}\boldsymbol{h}_{i},\boldsymbol{v}_{i} = W^{V}\boldsymbol{h}_{i}
\end{equation}

Note that $W^{Q}$, $W^{K}$ and $W^{V}$ are 128-to-128 linear projections.

After that, compatibility $u_{(c) j}$ is computed by the dot product of query and key, with masking mechanism (setting $-\infty$ not to select actions in $\boldsymbol{s}_{t-1}$). 


\begin{equation}
u_{(c) j}= \begin{cases}\frac{\mathbf{q}_{(c)}^{T} \mathbf{k}_{j}}{\sqrt{128}} & \text { if } j \notin \boldsymbol{s_{t-1}} \\ -\infty & \text { otherwise }\end{cases}
\label{mask1}
\end{equation}

The $tanh$ clipping is done following \citet{bello_pointer} and \citet{kool_attention}. 

\begin{equation}
    u_{(c) j}= \begin{cases}10 \cdot \tanh \left(\frac{\mathbf{q}_{(c)}^{T} \mathbf{k}_{j}}{\sqrt{128}}\right) & \text { if } j \notin \boldsymbol{s_{t-1}} \\ -\infty & \text { otherwise. }\end{cases}
\label{mask2}
\end{equation}

Finally, probability can be computed using softmax function as follows:

\begin{equation}
    p_{\boldsymbol{\theta}}\left(a_{t}=i \mid \boldsymbol{s}_{t-1} \right)=\frac{e^{u_{(c) i}}}{\sum_{j} e^{u_{(c) j}}}
\end{equation}
