# Supplementary material for: DevFormer: A Symmetric Transformer for Context-Aware Device Placement
Source: arXiv:2205.13225 source file (2023-06-07)
Supplement: Supplementary file 8 [file F_Ablation.tex]

This section reports ablation studies on action permutation invariance and hyperparameters $\lambda$, $P$, $N$. 


\subsection{Ablation Study on Action Permutation Invariance}
We measured the action permutation (AP) invariance of the model using $L_U$ in \eqref{L_U} for the test dataset. \cref{AP} shows that our CDML has an extremely lower AP invariant loss than that of AM-IL. This implies that \textit{SL aug} and \textit{USL aug} components in CDML contribute to learn AP invariance for our model and to performance increments as shown in \cref{components}.


\begin{table}[h!]
\fontsize{9}{9}\selectfont
\begin{center}
\caption{ Evaluation of action permutation invariant. }
\label{AP}
\begin{tabular}{lc}
\specialrule{1.0pt}{0pt}{4pt}
& AP invariant loss \\
\specialrule{0.5pt}{0pt}{4pt}
AM-IL ($N=2000$)& 8.70$\times 10^{-21}$ \\
CDML ($N=1000$) & 1.25$\times 10^{-28}$  \\
\specialrule{1.0pt}{0pt}{4pt}
\end{tabular}
\end{center}
\vspace{-6mm}
\end{table}



\subsection{Ablation Study on $\lambda$}
$\lambda$ refers to the weight of unsupervised loss term, $L_U$, in the semi-supervised learning loss \eqref{L}. To set $\lambda \times L_U$ be $0.1 \sim 1$, we first multiplied $10^{32}$ to $\lambda$ because probability of a specific solution is extremely small. Then, we ablated for $\lambda \in \{1,2,4,6,7,8,9,10 \}$ ($10^{32}$ is omitted) with fixed $N=100$, $P=3$. For every $\lambda$, it prevents overfitting of the model in comparison to baselines trained only with $L_{IL}$ (see Figure 17). The $\lambda = 8$ gives the best validation scores. However, the performance was not very sensitive to $\lambda$ compared to other ML baselines' performance. See \cref{Table01}.    

\begin{table}[h]
\fontsize{9}{9}\selectfont
\begin{center}
\caption{{Ablation study of $\lambda$ on fixed $P=3$ and $N=100$.}}\label{table_lambda}
\vspace{1mm}
\begin{tabular}{lc}
\specialrule{1.0pt}{0pt}{4pt}
$\lambda$ & Validation Score \\
\specialrule{0.5pt}{0pt}{4pt}
1& 12.96 \\
2 & 12.96 \\
4 & 12.94 \\
6 & 12.96 \\
7 & 12.98 \\
8 & \textbf{12.98} \\
9 & 12.97 \\
10 & 12.96 \\
\specialrule{0.5pt}{0pt}{4pt}
Only IL, $\lambda = 0$& 12.97 \\
\specialrule{1.0pt}{0pt}{4pt}
\label{table_lambda}
\end{tabular}
\end{center}
\end{table}

\begin{figure}[h]
\centerline{\includegraphics[width=0.5\textwidth]{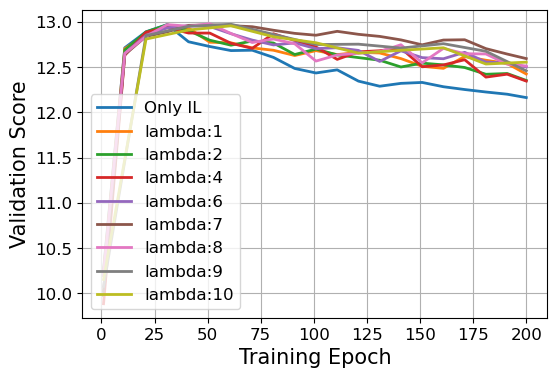}}
\caption{Validation graph of $\lambda \in \{1,2,4,6,7,8,9,10\}$ on fixed $P=3$ and $N=100$.}
\label{figure_lambda}
\end{figure}


\clearpage


\subsection{Ablation Study on $P$}
$P$ is the number of permutation transformed data of each expert data used for supervised learning. We ablate $P \in \{3,5,7\}$ with fixed $N=100$ and $\lambda=8$ and compare to only IL (supervised learning) training case (i.e., only with SL aug) verses semi-supervised learning case (i.e. SL auge + USL aug). As shown in \cref{table_P}, $P=3$ with \{SL aug + USL aug\} give best performances. For every $P$, \{SL aug + USL aug \} gives best performances. The performances is not very sensitive to $P$ to compare with other ML baselines' performance. See \cref{Table01}.    



\begin{table}[h]
\fontsize{9}{9}\selectfont
\begin{center}
\caption{{Ablation study on $P$ with and without unsupervised loss term.}}\label{table_P}
\vspace{1mm}
\begin{tabular}{lc}
\specialrule{1.0pt}{0pt}{4pt}
 & Validation Score \\
\specialrule{1.0pt}{0pt}{4pt}
SL aug \{$P=3$\}  & 12.97 \\ \rowcolor{Gray}
+ USL aug \{$\lambda = 8$\}& \textbf{12.98} \\
\specialrule{1.0pt}{0pt}{4pt}
SL aug \{$P=5$\} & 12.95 \\\rowcolor{Gray}
+ USL aug \{$\lambda = 8$\}& \textbf{12.95} \\
\specialrule{1.0pt}{0pt}{4pt}
SL aug \{$P=7$\} & 12.93 \\\rowcolor{Gray}
+ USL aug \{$\lambda = 8$\}& \textbf{12.95} \\
\specialrule{1.0pt}{0pt}{4pt}
\label{table_lambda}
\end{tabular}
\end{center}
\end{table}


\begin{figure}[h]
\centerline{\includegraphics[width=0.6\textwidth]{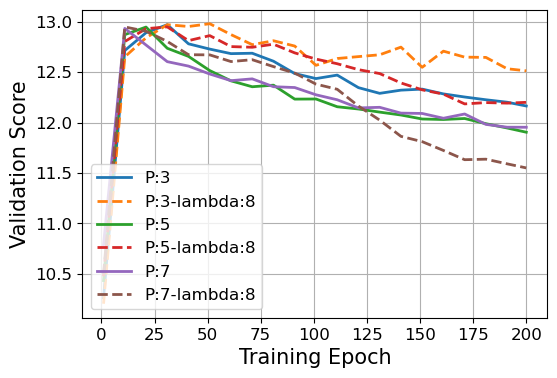}}
\caption{Validation score of $P$ ablation with and without Unsupervised Loss term.}
\label{figure_P}
\end{figure}


\clearpage

\subsection{Ablation Study on $N$}
$N$ is the number of expert data generated by the expert policy, GA $\{M=100\}$. We ablate $N \in \{100,500,1000,2000\}$ with fixed $P=3$ and $\lambda=8$ and compare with AM-IL baseline for all $N$. As shown in \cref{table_N}, CDML in $N=2000$ gives the best performances and CDML outperforms AM-IL for all $N$. Performance of the AM-IL is saturated at $N>500$ while the performance of CDML continuously increases as $N$ increases. 




\begin{table}[h]
\fontsize{9}{9}\selectfont
\begin{center}

\caption{{Ablation study on $N$ for CDML ($P=3, \lambda=8$) and AM-IL.}}\label{table_N}
\vspace{1mm}
\begin{tabular}{lc}
\specialrule{1.0pt}{0pt}{4pt}
 & Validation Score \\
\specialrule{1.0pt}{0pt}{4pt}
AM-IL \{$N=100$\}  & 11.60 \\ \rowcolor{Gray}
CDML (ours) \{$N=100$\}& \textbf{12.98} \\
\specialrule{1.0pt}{0pt}{4pt}
AM-IL \{$N=500$\}  & 12.37 \\ \rowcolor{Gray}
CDML (ours) \{$N=500$\}& \textbf{12.99} \\
\specialrule{1.0pt}{0pt}{4pt}
AM-IL \{$N=1000$\}  & 12.23 \\ \rowcolor{Gray}
CDML (ours) \{$N=1000$\}& \textbf{13.09} \\
\specialrule{1.0pt}{0pt}{4pt}
AM-IL \{$N=2000$\}  & 12.32 \\ \rowcolor{Gray}
CDML (ours) \{$N=2000$\}& \textbf{13.13} \\
\specialrule{1.0pt}{0pt}{4pt}


\label{table_lambda}

\end{tabular}
\end{center}
\end{table}



\begin{figure}[h]
\centerline{\includegraphics[width=0.6\textwidth]{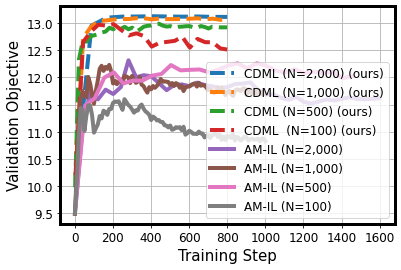}}
\caption{Validation score of CDML ($P=3, \lambda=8$) and AM-IL for $N \in \{100,500,1000,2000\}$.}
\label{figure_N}
\end{figure}
