# Supplementary material for: DevFormer: A Symmetric Transformer for Context-Aware Device Placement
Source: arXiv:2205.13225 source file (2023-06-07)
Supplement: Supplementary file 10 [file appendix_rel_work.tex]

\subsection{Machine Learning for Hardware Design}
With the CMOS technology shrink and increasing data rate, the design complexity of very large-scale integrated (VLSI) has increased. Human experts are no longer able to design hardware without the help of electrical design automation (EDA) tools, and EDA tools now suffer from time complexity of design and insufficient computing power, making ML application in hardware design inevitable. ML functionalities such as decision-making, performance prediction, black-box optimization and automated design play important roles in hardware design \citep{hardware_ml}. 


 However, ML methods with simplified objectives are in fact insufficient for practical hardware application. We took electrical performance in terms of power integrity (PI) as the objective of DPP, which requires complex computations, and devised the \ourmethod{} framework that successfully deals with such a complex objective. 


\subsection{Previous Works on DPP}
\textbf{Machine Learning-based Methods.}
Machine learning (ML) has become mainstream to solve DPP since the work of \citet{Qlearning_hyunwook} using Q-learning. Later, several approaches with convolutional neural network (CNN)-based Q approximator were proposed by \citet{doubleQ_lin}. However, their training sample efficiency is low, and their trained policies do not have reusability; if the problem changes, they must be re-trained. In an effort to overcome the reusability limitation, \citet{hyunwook_decap, pointer_haeyeon} implemented promising neural combinatorial optimization (NCO) models, by which a reusable policy capable of producing instant solutions to new problems without iterative exploration and domain knowledge can be constructed. However, their methods still showed poor sample efficiency and unsatisfactory performance.


\textbf{Genetic Algorithm-based Methods.} The most competitive non-learning method for DPP is the genetic algorithm (GA)  \citep{ga6, ga8, ga9, ga10}. GA is easy-to-implement in black-box optimization tasks. However, GA needs a massive iteration of objective evaluation per each problem to obtain a near-optimal solution. Therefore, outperforming GA without massive iteration of objective evaluation has become the main challenge for DPP.


\subsection{\textcolor{red}{Meta Learning and Offline Reinforcement Learning.}}
\textcolor{red}{Meta learning can simply be explained as learning to learn. Meta learning trains a model on several tasks for fast adaptation and transfers the model to new tasks. Meta learning can be categorized into gradient-based \citep{model-agnostic, on_first_order} and context-based methods \citep{memory-augmented, conditional_neural_processes}. }
Gradient-based methods find the meta-parameters by optimizing the task-adaptiveness on various tasks. For instance, \citet{model-agnostic} takes few-shot gradient descent on various tasks and finds the meta-parameters that best adapt to each task.

Context-based methods train meta-conditioned model by extracting shared contextual features between tasks through DNN and conditioning the model with the extracted contexts. For example, \citet{conditional_neural_processes} effectively reduced iterative process through context conditioning that allows fast task adaptation.

Our proposed \ourmethod{} is a \textit{context-based offline meta learning} method. \ourmethod{} trains a policy (i.e., DPP solver) with offline dataset consisting of various DPP tasks composed of different probing port and keep-out region. The probing port context network (PCN) encodes the probing port context and decoder learns the context-based meta features conditioned in PCN. Our method differs from the previous context-based meta learning methods in that meta learning process in \ourmethod{} is done through offline imitation learning.
%우리는 PCN을 통해 probing port 에 대한 정보를 encoding 하여, decoder가 PCN에 conditioned 된 context-based meta learning 을 수행한다. 다른 context meta learning 들과의 차이점은 바로 이 과정이 offline imitation learning을 통해서 이루어지는 점 이다. 
 


\subsection{Neural Combinatorial Optimization}
The field of neural combinatorial optimization (NCO) uses deep learning technology and aims to train a solver for classical combinatorial optimization problems such as travelling salesman problem (TSP) and its invariant problems \citep{vinyals_pointer,kool_attention}, vehicle routing problem and vertex cover problem. NCO methods automatically learn the heuristics to solve complex problems without human experts' domain knowledge. 

\textbf{Attention Model (AM) \citep{kool_attention}.} Attention Model (AM) is a representative NCO model that shows great performance on various combinatorial optimization problems, including hardware optimization \citep{liao2020attention} and DPP \citep{hyunwook_decap}. We observed that such performance of AM comes from (a) the expression power of transformer \citep{transformer} and (b) context embedding, which is used to capture meta level representation of the target problem. Therefore, we used the AM framework with a new context embedding for DPP adaptation.

\textbf{Relationship between DPP and NCO.} DPP task is categorized as a combinatorial optimization problem. Thus, implementing the existing classical NCO methods is very essential. However, there exist three major differences between DPP and classical CO; (a) optimal solution is not yet found, (b) a promising heuristic solver like Concorde does not exist and (c) objective evaluation of solution is complex; in TSP, measuring tour length is easy to compute. Therefore, promising machine learning techniques need to be devised to adapt classical NCO models to DPP and other hardware design tasks.      
